# Supplementary material for: Interaction-aware Conformal Prediction for Crowd Navigation
Source: arXiv:2502.06221 source file (2025-02-10)
Supplement: Supplementary file 1 [file Supplementary_Material.tex]

\begin{table*}[hbt!]
% \caption{Performance of ICP with and without Regularization. \textcolor{red}{How to measure the change of conformal prediction radius? Difference of initial and final radius? The ratio of conformal interval radius change with respect to the initial one?}}\label{table-quantitative}
\caption{Performance of ICP with and without Regularization. \textcolor{red}{To be moved to supplementary material if needed. Will not be discussed.}}\label{table-quantitative}
\begin{center}
\begin{tabular}{c|c|ccccccc}
    \hline
    Method & Reg & SR$\uparrow$ & ITR$\downarrow$ & SD$\uparrow$ & PL$\downarrow$ & NT$\downarrow$ & CR \\
    \hline
    ICP$_1$ & & 0.97 & 0.16$\pm$0.13 & 1.31$\pm$0.17 & 12.57$\pm$0.57 & 11.07$\pm$1.19 & 0.93$\pm$0.05 \\
    ICP$_1$ & $\checkmark$ & 0.98 & 0.15$\pm$0.12 & 1.32$\pm$0.16 & 12.59$\pm$0.67 & 11.12$\pm$1.25 & 0.93$\pm$0.05 \\
    \hline
\end{tabular}
\end{center}
\end{table*}
